# Supplementary material for: Solvation Entropy Made Simple
Source: arXiv:1901.11128 ancillary file (2019-01-30)
Supplement: Supplementary file 1 [file supporting_information.pdf]

# Supporting Information for "Solvation Entropy Made Simple"

Alejandro J. Garza*

*The Dow Chemical Company, 1776 Building Midland, Michigan 48674, United States*

E-mail: ajgarza@dow.com

Table 1: Solvent constants utilized in this work: mass density $\rho$ (g/mL), acentric factor $\omega$, relative permittivity $\epsilon_r$, and isobaric thermal expansion coefficient $\alpha$ ($10^{-3}$K$^{-1}$). In a few cases, $\alpha$ was not available and was assumed as zero due to its small impact on the entropy.

| Substance | $\rho$ | $\omega$ | $\epsilon_r$ | $\alpha$ |
|---|---|---|---|---|
| Ethylene | 0.57 | 0.089 | 1.0 | 2.40 |
| I2 | 3.96 | 0.229 | 4.0 | 0.00 |
| Cyclohexane | 0.778 | 0.212 | 2.0 | 1.21 |
| Benzene | 0.88 | 0.212 | 2.3 | 1.25 |
| Toluene | 0.867 | 0.263 | 2.4 | 1.08 |
| m-Xylene | 0.86 | 0.325 | 2.4 | 0.99 |
| o-Xylene | 0.88 | 0.31 | 2.6 | 0.00 |
| n-Pentane | 0.626 | 0.251 | 1.4 | 1.58 |
| Isopentane | 0.616 | 0.227 | 1.8 | 0.00 |
| n-Hexane | 0.66 | 0.299 | 1.9 | 1.41 |
| n-Octane | 0.703 | 0.398 | 2.0 | 1.14 |
| Chloroform | 1.49 | 0.218 | 4.8 | 1.27 |
| Dioxane | 0.796 | 0.307 | 2.3 | 1.12 |

| | | | | |
|---|---|---|---|---|
| Acetaldehyde | 0.788 | 0.303 | 21.1 | 1.69 |
| Acetone | 0.784 | 0.304 | 20.7 | 1.43 |
| Ethyl Acetate | 0.81 | 0.329 | 6.0 | 1.38 |
| Acetic Acid | 1.05 | 0.447 | 6.2 | 1.10 |
| Acetonitrile | 0.786 | 0.278 | 37.5 | 1.36 |
| Methyl Ether | 0.74 | 0.2 | 5.3 | 0.00 |
| Ethyl Ether | 0.713 | 0.281 | 4.3 | 1.60 |
| He | 0.13 | -0.365 | 1.1 | -1.49 |
| Ne | 1.21 | -0.029 | 1.5 | 15.40 |
| Ar | 1.40 | 0.001 | 1.5 | 4.80 |
| Kr | 2.41 | 0.005 | 1.7 | 0.00 |
| Xe | 2.94 | 0.008 | 1.9 | 0.00 |
| Water | 1 | 0.344 | 78.5 | 0.21 |
| Methanol | 0.796 | 0.556 | 32.6 | 1.09 |
| Ethanol | 0.796 | 0.644 | 24.6 | 1.09 |
| Propanol | 0.803 | 0.623 | 20.1 | 0.79 |
| Isopropanol | 0.786 | 0.665 | 17.9 | 0.00 |
| Butanol | 0.81 | 0.593 | 17.8 | 0.75 |
| Isobutanol | 0.802 | 0.592 | 17.3 | 0.94 |

Table 2: Experimental and calculated gas phase and solvation entropies (cal/mol-K) for 110 substances and mixtures. The conditions are $P = 1$ bar and $T = 298.15$ K except for pure noble gases and ethylene, for which the $T = T_b$.

| Solute | Solvent | $S^\circ_{\text{gas,exp}}$ | $S^\circ_{\text{gas,calc}}$ | $\Delta S^\circ_{\text{sol,exp}}$ | $\Delta S^\circ_{\omega}$ | $\Delta S^\circ_{\epsilon}$ | $\Delta S^\circ_{\epsilon\alpha}$ |
|---|---|---|---|---|---|---|---|
| Ethylene | Ethylene | 52.4 | -24.3 | 52.3 | -21.4 | -26.2 | -23.2 |
| $I_2$ | $I_2$ | 62.3 | -26.4 | 62.0 | -24.9 | -26.5 | -26.5 |
| Cyclohexane | Cyclohexane | 71.2 | -26.7 | 70.9 | -22.8 | -22.5 | -22.1 |

| | | | | | | | |
|---|---|---|---|---|---|---|---|
| Benzene | Benzene | 64.3 | -22.9 | 64.7 | -23.5 | -23.6 | -23.2 |
| Toluene | Toluene | 76.7 | -20.9 | 78.2 | -23.4 | -23.3 | -22.9 |
| m-Xylene | m-Xylene | 85.6 | -24.9 | 83.5 | -23.5 | -23.0 | -22.6 |
| o-Xylene | o-Xylene | 84.5 | -25.7 | 83.5 | -23.4 | -23.0 | -23.0 |
| n-Pentane | n-Pentane | 83.5 | -20.5 | 80.1 | -22.5 | -21.8 | -21.7 |
| Isopentane | Isopentane | 82.4 | -20.2 | 79.3 | -22.0 | -21.8 | -21.8 |
| n-Hexane | n-Hexane | 92.9 | -22.2 | 93.3 | -22.7 | -22.5 | -22.1 |
| n-Octane | n-Octane | 111.6 | -25.3 | 111.5 | -23.0 | -22.3 | -22.0 |
| Chloroform | Chloroform | 70.6 | -25.2 | 73.6 | -24.3 | -24.9 | -23.6 |
| Dioxane | Dioxane | 71.6 | -24.7 | 71.7 | -23.0 | -22.1 | -21.7 |
| Acetaldehye | Acetaldehyde | 59.8 | -31.8 | 60.1 | -26.1 | -27.9 | -24.9 |
| Acetone | Acetone | 70.6 | -22.7 | 66.6 | -25.1 | -27.1 | -24.6 |
| Ethyl Acetate | Ethyl Acetate | 86.6 | -24.7 | 85.0 | -23.5 | -24.7 | -23.2 |
| Acetic Acid | Acetic Acid | 67.6 | -29.8 | 69.1 | -27.9 | -26.7 | -25.6 |
| Acetonitrile | Acetonitrile | 62.4 | -26.6 | 57.9 | -26.2 | -28.5 | -25.8 |
| Methyl Ether | Methyl Ether | 55.7 | -20.7 | 60.6 | -23.9 | -25.3 | -25.3 |
| Ethyl Ether | Ethyl Ether | 81.7 | -21.2 | 82.6 | -23.4 | -24.4 | -23.2 |
| He | He | 8.1 | -4.7 | 9.0 | 0.1 | -3.4 | -3.4 |
| Ne | Ne | 35.0 | -17.9 | 35.0 | -18.0 | -17.3 | -17.3 |
| Ar | Ar | 37.0 | -18.4 | 37.0 | -21.0 | -19.8 | -19.6 |
| Kr | Kr | 39.2 | -18.6 | 39.2 | -21.5 | -20.3 | -20.3 |
| Xe | Xe | 40.5 | -18.8 | 40.6 | -21.8 | -20.8 | -20.8 |
| Water | Water | 45.1 | -28.4 | 45.1 | -31.1 | -32.4 | -31.9 |
| Methanol | Methanol | 57.3 | -26.9 | 56.6 | -30.2 | -29.4 | -27.3 |
| Ethanol | Ethanol | 67.6 | -29.4 | 64.9 | -29.8 | -28.2 | -26.1 |
| Propanol | Propanol | 77.0 | -31.0 | 74.2 | -28.6 | -27.3 | -25.9 |
| Isopropanol | Isopropanol | 79.6 | -33.5 | 72.5 | -28.9 | -26.9 | -26.9 |

| | | | | | | | |
|---|---|---|---|---|---|---|---|
| Butanol | Butanol | 86.5 | -32.5 | 83.0 | -27.5 | -26.7 | -25.4 |
| Isobutanol | Isobutanol | 83.6 | -32.4 | 82.2 | -27.4 | -26.2 | -24.6 |
| Acetic Acid | Water | 67.6 | -25.4 | 69.1 | -30.2 | -29.0 | -28.1 |
| Methanol | Water | 57.3 | -27.2 | 56.6 | -26.4 | -26.9 | -26.2 |
| Ethanol | Water | 67.6 | -31.6 | 64.9 | -30.3 | -28.9 | -28.0 |
| Propanol | Water | 77.0 | -33.1 | 74.2 | -32.7 | -30.5 | -29.5 |
| Isopropanol | Water | 79.6 | -30.5 | 72.5 | -32.5 | -30.3 | -29.2 |
| Butanol | Water | 86.5 | -35.1 | 83.4 | -35.5 | -32.2 | -31.0 |
| Acetonitrile | Water | 62.4 | -22.9 | 57.9 | -28.4 | -27.9 | -27.1 |
| Ethyl Ether | Water | 81.7 | -31.3 | 82.6 | -36.6 | -32.6 | -31.4 |
| Acetaldehyde | Water | 59.8 | -28.5 | 60.1 | -28.7 | -28.1 | -27.3 |
| Acetone | Water | 70.6 | -28.5 | 67.9 | -31.9 | -29.8 | -28.8 |
| Ethylene | Water | 52.4 | -22.6 | 52.3 | -26.4 | -27.4 | -26.6 |
| H | Water | 27.4 | -16.9 | 27.4 | -18.6 | -20.4 | -20.1 |
| He | Water | 30.1 | -17.1 | 30.2 | -19.8 | -21.6 | -21.2 |
| Ne | Water | 35.0 | -19.6 | 35.0 | -21.1 | -22.9 | -22.4 |
| Ar | Water | 37.0 | -23.0 | 37.0 | -22.5 | -23.9 | -23.3 |
| Kr | Water | 39.2 | -23.2 | 39.2 | -23.3 | -24.4 | -23.7 |
| Xe | Water | 40.5 | -23.5 | 40.6 | -24.2 | -25.0 | -24.2 |
| $I_2$ | Water | 62.3 | -27.1 | 62.0 | -28.4 | -28.4 | -27.5 |
| $CO_2$ | Water | 51.1 | -26.5 | 50.3 | -24.9 | -26.1 | -25.4 |
| Cyclopentane | Water | 72.2 | -32.0 | 73.7 | -33.8 | -31.2 | -30.1 |
| Cyclohexane | Water | 71.2 | -31.6 | 70.9 | -36.1 | -32.4 | -31.1 |
| Xenon | n-Hexane | 40.5 | -10.7 | 40.5 | -13.3 | -13.4 | -13.2 |
| Xenon | n-Octane | 40.5 | -10.6 | 40.5 | -12.7 | -12.7 | -12.6 |
| Xenon | Ethanol | 40.5 | -11.2 | 40.5 | -19.7 | -19.7 | -17.9 |
| Xenon | Butanol | 40.5 | -11.3 | 40.5 | -16.5 | -17.2 | -16.3 |

| | | | | | | | |
|---|---|---|---|---|---|---|---|
| 1,4-Dioxane | Ethanol | 71.6 | -17.1 | 71.7 | -25.1 | -23.5 | -20.9 |
| n-Octane | Ethanol | 111.6 | -19.7 | 111.5 | -32.8 | -27.0 | -23.6 |
| Toluene | Ethanol | 76.7 | -19.4 | 78.2 | -27.0 | -24.5 | -21.7 |
| Nitromethane | Ethanol | 71.7 | -17.5 | 67.4 | -23.3 | -22.2 | -20.2 |
| Methanol | Butanol | 57.3 | -20.8 | 56.6 | -18.2 | -18.7 | -17.9 |
| Ethanol | Butanol | 67.6 | -23.4 | 64.9 | -20.3 | -20.1 | -19.1 |
| Benzene | Butanol | 64.3 | -20.1 | 64.7 | -21.8 | -21.7 | -20.4 |
| Toluene | Butanol | 76.7 | -20.0 | 78.2 | -22.8 | -22.3 | -20.9 |
| n-Octane | Butanol | 111.6 | -22.9 | 111.5 | -26.5 | -24.3 | -22.6 |
| Butanol | Benzene | 86.5 | -19.6 | 83.0 | -18.7 | -19.0 | -18.5 |
| Pentanol | Benzene | 95.9 | -20.8 | 92.2 | -19.3 | -19.5 | -19.0 |
| Cyclohexane | Benzene | 71.2 | -16.4 | 70.9 | -18.6 | -18.6 | -18.1 |
| n-Pentane | Benzene | 83.5 | -14.1 | 85.6 | -18.9 | -19.1 | -18.6 |
| Toluene | Benzene | 76.7 | -18.7 | 78.2 | -19.1 | -19.1 | -18.6 |
| Ethanol | Benzene | 67.6 | -18.6 | 64.9 | -17.3 | -17.8 | -17.4 |
| Ethanol | Toluene | 67.6 | -17.6 | 64.9 | -16.8 | -17.2 | -16.8 |
| Propanol | Toluene | 77.0 | -18.9 | 74.2 | -17.9 | -18.1 | -17.7 |
| Butanol | Toluene | 86.5 | -21.7 | 83.0 | -18.6 | -18.7 | -18.3 |
| Pentanol | Toluene | 95.9 | -22.6 | 92.2 | -19.2 | -19.2 | -18.8 |
| Acetone | Toluene | 70.6 | -18.4 | 66.6 | -17.4 | -17.7 | -17.3 |
| Butanone | Toluene | 74.1 | -19.8 | 75.2 | -18.5 | -18.7 | -18.3 |
| 1,4-Dioxane | Toluene | 71.6 | -20.6 | 71.7 | -18.3 | -18.3 | -17.9 |
| n-Octane | Toluene | 111.6 | -16.8 | 111.5 | -20.5 | -20.1 | -19.6 |
| Acetonitrile | Cyclohexane | 62.4 | -14.5 | 57.9 | -16.2 | -16.4 | -16.1 |
| Ethanol | Cyclohexane | 67.6 | -12.3 | 64.9 | -16.7 | -16.9 | -16.6 |
| Propanol | Cyclohexane | 77.0 | -15.3 | 74.2 | -17.7 | -17.8 | -17.5 |
| Butanol | Cyclohexane | 86.5 | -16.8 | 83.0 | -18.5 | -18.4 | -18.1 |

| | | | | | | | |
|---|---|---|---|---|---|---|---|
| Pentanol | Cyclohexane | 95.9 | -19.8 | 92.2 | -19.1 | -18.9 | -18.5 |
| Hexanol | Cyclohexane | 105.0 | -17.7 | 100.9 | -19.7 | -19.3 | -18.9 |
| Ethyl Acetate | Cyclohexane | 86.6 | -16.8 | 85.0 | -19.0 | -18.8 | -18.5 |
| Diethyl Ether | Cyclohexane | 81.7 | -14.7 | 82.6 | -18.9 | -18.8 | -18.5 |
| 1,4-Dioxane | Cyclohexane | 71.6 | -17.2 | 71.7 | -18.2 | -18.0 | -17.7 |
| Benzene | Cyclohexane | 64.3 | -16.9 | 64.7 | -18.4 | -18.3 | -17.9 |
| Toluene | Cyclohexane | 76.7 | -18.0 | 78.2 | -18.8 | -18.6 | -18.2 |
| Ethanol | n-Hexane | 67.6 | -12.7 | 64.9 | -15.5 | -15.7 | -15.4 |
| Butanol | n-Hexane | 86.5 | -16.6 | 83.0 | -17.0 | -17.0 | -16.7 |
| Hexanol | n-Hexane | 105.0 | -16.7 | 100.9 | -18.9 | -18.6 | -18.2 |
| 1,4-Dioxane | n-Hexane | 71.6 | -17.7 | 71.7 | -16.7 | -16.6 | -16.3 |
| Nitromethane | n-Hexane | 71.7 | -14.8 | 67.5 | -15.2 | -15.4 | -15.1 |
| Acetone | n-Hexane | 70.6 | -15.2 | 66.6 | -15.9 | -16.0 | -15.7 |
| Butanone | n-Hexane | 74.1 | -16.7 | 75.2 | -16.8 | -16.8 | -16.4 |
| Chloroform | n-Hexane | 70.6 | -19.7 | 71.7 | -15.6 | -15.7 | -15.4 |
| Toluene | n-Hexane | 76.7 | -17.5 | 78.2 | -17.8 | -17.6 | -17.3 |
| Benzene | n-Hexane | 64.3 | -17.7 | 64.7 | -16.8 | -16.7 | -16.4 |
| Toluene | Chloroform | 76.7 | -20.9 | 78.2 | -20.4 | -20.7 | -19.4 |
| Ethanol | Chloroform | 67.6 | -19.4 | 64.9 | -18.3 | -19.0 | -18.0 |
| Propanol | Chloroform | 77.0 | -19.8 | 74.2 | -19.5 | -20.1 | -19.0 |
| Butanol | Chloroform | 86.5 | -22.3 | 83.0 | -20.1 | -20.5 | -19.3 |
| Hexanol | Chloroform | 105.0 | -24.4 | 100.9 | -21.7 | -21.7 | -20.3 |
| n-Octane | Chloroform | 111.6 | -18.9 | 111.5 | -22.7 | -22.4 | -20.8 |
| Acetone | Chloroform | 70.6 | -23.1 | 66.6 | -19.3 | -19.9 | -18.8 |
| Ethyl Acetate | Chloroform | 86.6 | -22.8 | 85.0 | -20.5 | -20.9 | -19.7 |
| Benzene | Chloroform | 64.3 | -19.8 | 64.7 | -19.8 | -20.3 | -19.1 |

Table 3: Experimental and calculated vaporization enthalpies (kcal/mol) for 32 substances at their boiling point.

| Substance | $T_b/K$ | $\Delta H_{\text{vap}}^{\text{exp}}$ | $T_b\Delta S_\omega$ | $T_b\Delta S_\epsilon$ | $T_b\Delta S_{\epsilon\alpha}$ |
|---|---|---|---|---|---|
| Ethylene | 169.40 | 4.12 | 3.62 | 3.63 | 3.62 |
| $I_2$ | 457.4 | 9.93 | 12.14 | 12.88 | 12.88 |
| Cyclohexane | 353.9 | 9.45 | 8.29 | 8.20 | 8.04 |
| Benzene | 353.20 | 7.35 | 8.54 | 8.58 | 8.38 |
| Toluene | 383.8 | 8.00 | 9.36 | 9.33 | 9.12 |
| m-Xylene | 412.2 | 8.96 | 10.20 | 10.00 | 9.78 |
| o-Xylene | 417.20 | 8.66 | 10.33 | 10.14 | 10.14 |
| n-Pentane | 309.2 | 6.49 | 7.01 | 6.79 | 6.74 |
| Isopentane | 301 | 5.90 | 6.62 | 6.55 | 6.55 |
| n-Hexane | 341.20 | 7.41 | 7.92 | 7.84 | 7.69 |
| n-Octane | 398.2 | 9.79 | 9.62 | 9.35 | 9.17 |
| Chloroform | 334.35 | 8.43 | 8.12 | 8.31 | 7.90 |
| Dioxane | 374.2 | 9.08 | 8.95 | 8.60 | 8.40 |
| Acetaldehyde | 293.3 | 6.16 | 7.64 | 8.16 | 7.29 |
| Acetone | 329.2 | 7.47 | 8.38 | 9.05 | 8.12 |
| Ethyl Acetate | 350.2 | 8.38 | 8.46 | 8.86 | 8.28 |
| Acetic Acid | 391.2 | 12.02 | 11.34 | 10.87 | 10.28 |
| Acetonitrile | 355.2 | 9.45 | 9.54 | 10.38 | 9.23 |
| Methyl Ether | 248.34 | 5.14 | 5.92 | 6.29 | 6.29 |
| Ethyl Ether | 307.8 | 7.10 | 7.24 | 7.55 | 7.16 |
| He | 4.20 | 0.02 | 0.00 | 0.01 | 0.01 |
| Ne | 27.10 | 0.49 | 0.49 | 0.47 | 0.46 |
| Ar | 87.30 | 1.61 | 1.84 | 1.73 | 1.71 |
| Kr | 115.75 | 2.15 | 2.49 | 2.35 | 2.35 |

| | | | | | |
|---|---|---|---|---|---|
| Xe | 165.00 | 3.10 | 3.60 | 3.44 | 3.44 |
| Water | 373.2 | 9.74 | 11.92 | 12.41 | 12.20 |
| Methanol | 337.8 | 9.12 | 10.36 | 10.10 | 9.28 |
| Ethanol | 351.5 | 9.21 | 10.70 | 10.13 | 9.29 |
| Propanol | 370.2 | 11.20 | 10.91 | 10.43 | 9.79 |
| Isopropanol | 355.8 | 10.54 | 10.54 | 9.83 | 9.83 |
| Butanol | 390.8 | 10.34 | 11.17 | 10.84 | 10.19 |
| Isobutanol | 381.2 | 9.99 | 10.83 | 10.37 | 9.59 |

# References


(1) Lucius, J.E.; Olhoeft, G.R.; Hill, P.L.; Duke, S.K. Properties and hazards of 108 selected substances–1992 edition. *US Geological Survey Open-File Report* **1992**, *92*, 527–554.

(2) Dionísio, M.S.; Ramos, J.J.M.; Gonçalves, R.M. The Enthalpy and Entropy of Cavity Formation in Liquids and Corresponding States Principle. *Can. J. Chem.* **1990**, *68*, 1937–1949.

(3) P.J. Linstrom and W.G. Mallard, Eds., NIST Chemistry WebBook, NIST Standard Reference Database Number 69, National Institute of Standards and Technology, Gaithersburg MD, 20899, https://doi.org/10.18434/T4D303, (retrieved October 29, 2018).

(4) Sander, R. Compilation of Henry's Law Constants (version 4.0) for Water as Solvent. *Atmospheric Chem. Phys.* **2015** *15*, 4399–4981.

(5) Chickos, J.S.; Acree Jr, W.E. Enthalpies of Vaporization of Organic and Organometallic Compounds, 1880–2002. *J. Phys. Chem. Ref. Data* **2003** *32*, 519–878.

(6) Marenich, A.V.; Cramer, C.J.; Truhlar, D.G. Universal Solvation Model Based on

the Generalized Born Approximation with Asymmetric Descreening. *J. Chem. Theory Comput.* **2009** *5*, 2447-2464.

(7) Pollack, G.L.; Himm, J.F., 1982. Solubility of Xenon in Liquid n-Alkanes: Temperature Dependence and Thermodynamic Functions. *J. Chem. Phys.* **1982**, *77*, 3221–3229.

(8) Pollack, G.L.; Himm, J.F.; Enyeart, J.J. Solubility of Xenon in Liquid n-Alkanols: Thermodynamic Functions in Simple Polar Liquids. *J. Chem. Phys.* **1984**, *81*, 3239–3246.
